# Supplementary material for: Zero-Shot Learning for Requirements Classification: An Exploratory Study
Source: arXiv:2302.04723 source file (2023-03-15)
Supplement: Supplementary file 1 [file NFRmultiLabels.tex]

\begin{table}
\centering
\caption{Label configurations for all the NFR classes for the multi-class and multi-label classification sub-tasks in Task NFR (cf. Table \ref{tab:labelsNFRmulti})}
 \label{tab:appendixNFRmultiLabels}
  \resizebox{1\textwidth}{!}{
\begin{tabular}{lll} 
\toprule
\textbf{Label Abbr.}          & \textbf{Label Configuration}                                                          & \textbf{List of Labels}                                                                                                                                                                                                                                                                                                                                                                                                                                                                                                                                                                                                                                                                                                                                                                                                                                                                                                                                                                                                                                                                                                                                                                                                                                                                                                                                                                                                                                                                                                                                                                                                                                                                                                                                                                                                                                                                                                                                                                                                                                                                                                                                                                                                                                                          \\ 
\hline
\textbf{\textit{MultiNFR\_A}} & Original                                                                              & {[}"usability", "security", "performance", "operational", "look \& feel", "legal", "fault tolerance", "maintainability", scalability" availability"]                                                                                                                                                                                                                                                                                                                                                                                                                                                                                                                                                                                                                                                                                                                                                                                                                                                                                                                                                                                                                                                                                                                                                                                                                                                                                                                                                                                                                                                                                                                                                                                                                                                                                                                                                                                                                                                                                                                                                                                                                                                                                                                             \\
\textbf{\textit{MultiNFR\_B}} & Expert curated                                                                        & \begin{tabular}[c]{@{}l@{}}{[}"instructive, easy, helpful, useful, learnable, explainable, affordable, intuitive, or understandable",\\"security, authorization, or protection", "periodic execution or efficacy performance",\\"working, running, connecting, interfacing, or operative environment",\\"appearance, interface, look \& feel", "legal, law, or rules", "system recovery \& fault tolerance",\\"maintaining, fixing, running or updating", "scalable, increasable or developable", "avaliable or timely achievable"]\end{tabular}                                                                                                                                                                                                                                                                                                                                                                                                                                                                                                                                                                                                                                                                                                                                                                                                                                                                                                                                                                                                                                                                                                                                                                                                                                                                                                                                                                                                                                                                                                                                                                                                                                                                                                                                 \\
\textbf{\textit{MultiNFR\_C}} & \begin{tabular}[c]{@{}l@{}}Word Embedding \\(selected from top 20 words)\end{tabular} & \begin{tabular}[c]{@{}l@{}}{[}"accessibility, aesthetic, contextual, experience, satisfaction, HCI, UX, questionnaire, ease, or ergonomics" ,\\"vulnerability, securing. protecting, protection, cybersecurity, assurance, cyber, countermeasure, threat, \\privacy, authentication, prevention, or confidentiality",~"throughput, reliability, scalability, responsiveness, \\efficiency, workload, benchmark, latency, speed, improvement, or accuracy", "environmental, organizational, \\coordination, systemic, or logistics", "graphical, gui, ui, widget, interaction, habit, prefer, comfortable,\\~friendly, feeling, experience, or familiar", "liability, litigation, jurisdiction, regulation, copyright, legislation, \\enforcement, governmental, directive,civil, right, patentability, claim, violate, infringement, or counsel",\\"tolerance, failure, tolerant, byzantine, deadlock, exploiting, reliability, isolation, fault, guarantee, or dependable",\\"adaptability, effectiveness, agility, preventive, or dependability", "flexibility, workload, efficiency, or optimize",\\"reliability, dependability, resilience"]\end{tabular}                                                                                                                                                                                                                                                                                                                                                                                                                                                                                                                                                                                                                                                                                                                                                                                                                                                                                                                                                                                                                                                                                                                    \\
\textbf{\textit{MultiNFR\_D}} & \begin{tabular}[c]{@{}l@{}}Word Embedding\\~(selected from top 50 words)\end{tabular} & \begin{tabular}[c]{@{}l@{}}{[}"accessibility, aesthetic, contextual, experience, satisfaction, HCI, UX, questionnaire, ease, \\ergonomics, designer, evaluate, multimodal, practitioner, prototyping, preference, personalization,\\~suitability, focus, clarity, responsiveness, judgement, feel, or helpful" , "vulnerability, security, \\protection, cybersecurity, assurance, countermeasure, threat, privacy, authentication, prevention, \\confidentiality, trusted, intrusion, compromise, safety, insecure, defensive, breach, proactive, tampering, \\penetration, policy, phishing, vulnerable, authorization, dependability, or certification",\\"throughput, reliability, scalability, responsiveness, efficiency, workload, benchmark, latency, \\speed, improvement, accuracy, achieve, tuning, bottleneck, better, high, optimize, effectiveness, \\low, enhances, reducing, incresaed, quality, faster, or degrades", "environmental, organizational, \\coordination, systemic, logistics, coordination, or automation",~"graphical, gui, ui, widget, interaction, \\habit, prefer, comfortable, friendly, feeling, experience, familiar, desire, customize, intent, disability, or impression",\\"liability, litigation, jurisdiction, regulation, copyright, legislation, enforcement, governmental, directive,civil, right,\\~patentability, claim, violate, infringement, counsel, holder, dispute, illegal, judicial, ruling, agreement, ownership,\\~comply, authority, law, accountability, abuse, intellectual, obligation, invention, court, ethical, concern, or policy",\\"tolerance, failure, tolerant, byzantine, deadlock, exploiting, reliability, isolation, fault, guarantee, dependable, \\countermeasure, resilience, defensive, corruption, weakness, malfunction, robustness, or stability",\\"adaptability, effectiveness, agility, preventive, dependability, correcting, reuse, defect, mitigation, validated,\\~resilience, achievable, remedy, assessing, or maintaining",\\"flexibility, workload, efficiency, optimize, caching, improvement, robust, overhead, adaptability, scalable, or increased",\\"reliability, dependability, resilience, flexibility, accountability, ensur, disruption, timely, or standby"]\end{tabular}  \\
\bottomrule
\end{tabular}
}
\end{table}
