# Supplementary material for: Zero-Shot Learning for Requirements Classification: An Exploratory Study
Source: arXiv:2302.04723 source file (2023-03-15)
Supplement: Supplementary file 2 [file SUPPLEMENTARY-TopNFRbinaryResults.tex]

\begin{table}
\centering
\setlength{\extrarowheight}{0pt}
\addtolength{\extrarowheight}{\aboverulesep}
\addtolength{\extrarowheight}{\belowrulesep}
\setlength{\aboverulesep}{0pt}
\setlength{\belowrulesep}{0pt}

\caption{Binary classification results for top four NFR classes in \textit{Task NFR}.}
\label{tab:TopNFRbinresults}

  \resizebox{1\textwidth}{!}{
\begin{tabular}{l|ccc|ccc|ccc|ccc} 
\toprule
\multicolumn{1}{c|}{\multirow{2}{*}{\textbf{ZSL Classifier}}}         & \multicolumn{3}{c|}{\vcell{\textbf{US}}}                                          & \multicolumn{3}{c|}{\vcell{\textbf{SE}}}                                           & \multicolumn{3}{c|}{\vcell{\textbf{O}}}                                         & \multicolumn{3}{c}{\vcell{\textbf{PE}}}                                          \\[-\rowheight]
\multicolumn{1}{c|}{}                                                 & \multicolumn{3}{c|}{\printcelltop}                                                            & \multicolumn{3}{c|}{\printcelltop}                                                            & \multicolumn{3}{c|}{\printcelltop}                                                            & \multicolumn{3}{c}{\printcelltop}                                                              \\ 
\cline{2-13}
\multicolumn{1}{c|}{}                                                 & \vcell{\textbf{wP}}        & \vcell{\textbf{wR}}         & \vcell{\textbf{wF1}}        & \vcell{\textbf{wP}}        & \vcell{\textbf{wR}}         & \vcell{\textbf{wF1}}        & \vcell{\textbf{wP}}        & \vcell{\textbf{wR}}         & \vcell{\textbf{wF1}}        & \vcell{\textbf{wP}}        & \vcell{\textbf{wR}}         & \vcell{\textbf{wF1}}         \\[-\rowheight]
\multicolumn{1}{c|}{}                                                 & \printcelltop                 & \printcelltop                 & \printcelltop                 & \printcelltop                 & \printcelltop                 & \printcelltop                 & \printcelltop                 & \printcelltop                 & \printcelltop                 & \printcelltop                 & \printcelltop                 & \printcelltop                  \\ 
\hline
%\rowcolor[rgb]{0.867,0.867,0.867} 
\vcell{\textbf{Sbert + (NFR)\_A}}   & \vcell{0.74}                  & \vcell{0.40}                  & \vcell{0.37}                  & \vcell{0.49}                  & \vcell{0.28}                  & \vcell{0.18}                  & \vcell{0.79}                  & \vcell{0.45}                  & \vcell{0.44}                  & \vcell{0.76}                  & \vcell{0.39}                  & \vcell{0.39}                   \\[-\rowheight]
%\rowcolor[rgb]{0.867,0.867,0.867} 
\printcelltop                       & \printcelltop                 & \printcelltop                 & \printcelltop                 & \printcelltop                 & \printcelltop                 & \printcelltop                 & \printcelltop                 & \printcelltop                 & \printcelltop                 & \printcelltop                 & \printcelltop                 & \printcelltop                  \\
%\rowcolor[rgb]{0.867,0.867,0.867} 
\vcell{\textbf{Sbert + (NFR)\_B}}   & \vcell{0.71}                  & \vcell{0.43}                  & \vcell{0.42}                  & \vcell{0.35}                  & \vcell{0.24}                  & \vcell{0.17}                  & \vcell{0.78}                  & \vcell{0.43}                  & \vcell{0.42}                  & \vcell{0.75}                  & \vcell{0.36}                  & \vcell{0.35}                   \\[-\rowheight]
%\rowcolor[rgb]{0.867,0.867,0.867} 
\printcelltop                       & \printcelltop                 & \printcelltop                 & \printcelltop                 & \printcelltop                 & \printcelltop                 & \printcelltop                 & \printcelltop                 & \printcelltop                 & \printcelltop                 & \printcelltop                 & \printcelltop                 & \printcelltop                  \\
%\rowcolor[rgb]{0.867,0.867,0.867} 
\vcell{\textbf{Sbert + (NFR)\_C}}   & \vcell{0.74}                  & \vcell{0.43}                  & \vcell{0.41}                  & \vcell{0.34}                  & \vcell{0.22}                  & \vcell{0.19}                  & \vcell{0.80}                  & \vcell{0.45}                  & \vcell{0.44}                  & \vcell{0.76}                  & \vcell{0.38}                  & \vcell{0.38}                   \\[-\rowheight]
%\rowcolor[rgb]{0.867,0.867,0.867} 
\printcelltop                       & \printcelltop                 & \printcelltop                 & \printcelltop                 & \printcelltop                 & \printcelltop                 & \printcelltop                 & \printcelltop                 & \printcelltop                 & \printcelltop                 & \printcelltop                 & \printcelltop                 & \printcelltop                  \\
%\rowcolor[rgb]{0.867,0.867,0.867} 
\vcell{\textbf{Sbert + (NFR)\_D}}   & \vcell{0.77}                  & \vcell{0.78}                  & \vcell{0.78}                  & \vcell{\textbf{0.72}}         & \vcell{\textbf{0.71}}         & \vcell{\textbf{0.72}}         & \vcell{\textbf{0.68}}         & \vcell{\textbf{0.72}}         & \vcell{\textbf{0.70}}         & \vcell{0.80}                  & \vcell{0.67}                  & \vcell{0.70}                   \\[-\rowheight]
%\rowcolor[rgb]{0.867,0.867,0.867} 
\printcelltop                       & \printcelltop                 & \printcelltop                 & \printcelltop                 & \printcelltop                 & \printcelltop                 & \printcelltop                 & \printcelltop                 & \printcelltop                 & \printcelltop                 & \printcelltop                 & \printcelltop                 & \printcelltop                  \\
%\rowcolor[rgb]{0.867,0.867,0.867} 
\vcell{\textbf{Sbert + (NFR)\_E}}   & \vcell{\textbf{\uline{0.81}}} & \vcell{\textbf{\uline{0.82}}} & \vcell{\textbf{\uline{0.80}}} & \vcell{\textbf{0.76}}         & \vcell{\textbf{0.78}}         & \vcell{\textbf{0.75}}         & \vcell{0.68}                  & \vcell{0.63}                  & \vcell{0.65}                  & \vcell{\textbf{0.78}}         & \vcell{\textbf{\uline{0.78}}} & \vcell{\textbf{\uline{0.78}}}  \\[-\rowheight]
%\rowcolor[rgb]{0.867,0.867,0.867} 
\printcelltop                       & \printcelltop                 & \printcelltop                 & \printcelltop                 & \printcelltop                 & \printcelltop                 & \printcelltop                 & \printcelltop                 & \printcelltop                 & \printcelltop                 & \printcelltop                 & \printcelltop                 & \printcelltop                  \\
\hline
\vcell{\textbf{AllMini + (NFR)\_A}}                                   & \vcell{0.73}                  & \vcell{0.62}                  & \vcell{0.64}                  & \vcell{0.72}                  & \vcell{0.50}                  & \vcell{0.51}                  & \vcell{0.54}                  & \vcell{0.43}                  & \vcell{0.47}                  & \vcell{0.73}                  & \vcell{0.59}                  & \vcell{0.63}                   \\[-\rowheight]
\printcelltop                                                         & \printcelltop                 & \printcelltop                 & \printcelltop                 & \printcelltop                 & \printcelltop                 & \printcelltop                 & \printcelltop                 & \printcelltop                 & \printcelltop                 & \printcelltop                 & \printcelltop                 & \printcelltop                  \\
\vcell{\textbf{AllMini + (NFR)\_B}}                                   & \vcell{0.54}                  & \vcell{0.35}                  & \vcell{0.35}                  & \vcell{0.73}                  & \vcell{0.73}                  & \vcell{0.73}                  & \vcell{\textbf{0.71}}         & \vcell{\textbf{0.65}}         & \vcell{\textbf{0.67}}         & \vcell{\textbf{\uline{0.80}}} & \vcell{\textbf{0.70}}         & \vcell{\textbf{\uline{0.78}}}  \\[-\rowheight]
\printcelltop                                                         & \printcelltop                 & \printcelltop                 & \printcelltop                 & \printcelltop                 & \printcelltop                 & \printcelltop                 & \printcelltop                 & \printcelltop                 & \printcelltop                 & \printcelltop                 & \printcelltop                 & \printcelltop                  \\
\vcell{\textbf{AllMini + (NFR)\_C}}                                   & \vcell{0.31}                  & \vcell{0.23}                  & \vcell{0.17}                  & \vcell{0.59}                  & \vcell{0.65}                  & \vcell{0.61}                  & \vcell{0.67}                  & \vcell{0.58}                  & \vcell{0.61}                  & \vcell{0.68}                  & \vcell{0.57}                  & \vcell{0.60}                   \\[-\rowheight]
\printcelltop                                                         & \printcelltop                 & \printcelltop                 & \printcelltop                 & \printcelltop                 & \printcelltop                 & \printcelltop                 & \printcelltop                 & \printcelltop                 & \printcelltop                 & \printcelltop                 & \printcelltop                 & \printcelltop                  \\
\vcell{\textbf{AllMini + (NFR)\_D}}                                   & \vcell{\textbf{0.75}}         & \vcell{\textbf{0.75}}         & \vcell{\textbf{0.75}}         & \vcell{\textbf{\uline{0.84}}} & \vcell{\textbf{\uline{0.84}}} & \vcell{\textbf{\uline{0.84}}} & \vcell{0.65}                  & \vcell{0.55}                  & \vcell{0.58}                  & \vcell{0.81}                  & \vcell{0.69}                  & \vcell{0.71}                   \\[-\rowheight]
\printcelltop                                                         & \printcelltop                 & \printcelltop                 & \printcelltop                 & \printcelltop                 & \printcelltop                 & \printcelltop                 & \printcelltop                 & \printcelltop                 & \printcelltop                 & \printcelltop                 & \printcelltop                 & \printcelltop                  \\
\vcell{\textbf{AllMini + (NFR)\_E}}                                   & \vcell{0.69}                  & \vcell{0.71}                  & \vcell{0.69}                  & \vcell{0.73}                  & \vcell{0.72}                  & \vcell{0.73}                  & \vcell{0.60}                  & \vcell{0.54}                  & \vcell{0.57}                  & \vcell{0.75}                  & \vcell{0.73}                  & \vcell{0.74}                   \\[-\rowheight]
\printcelltop                                                         & \printcelltop                 & \printcelltop                 & \printcelltop                 & \printcelltop                 & \printcelltop                 & \printcelltop                 & \printcelltop                 & \printcelltop                 & \printcelltop                 & \printcelltop                 & \printcelltop                 & \printcelltop                  \\
\hline
%\rowcolor[rgb]{0.867,0.867,0.867} 
\vcell{\textbf{Bert4RE + (NFR)\_A}} & \vcell{\textit{0.53}}         & \vcell{\textit{0.73}}         & \vcell{\textit{0.62}}        & \vcell{\textit{0.59}}         & \vcell{\textit{0.70}}         & \vcell{\textit{0.62}}        & \vcell{\textit{0.56}}         & \vcell{\textit{0.75}}         & \vcell{\textit{0.64}}        & \vcell{0.61}                  & \vcell{0.58}                  & \vcell{0.59}                   \\[-\rowheight]
%\rowcolor[rgb]{0.867,0.867,0.867} 
\printcelltop                       & \printcelltop                 & \printcelltop                 & \printcelltop                 & \printcelltop                 & \printcelltop                 & \printcelltop                 & \printcelltop                 & \printcelltop                 & \printcelltop                 & \printcelltop                 & \printcelltop                 & \printcelltop                  \\
%\rowcolor[rgb]{0.867,0.867,0.867} 
\vcell{\textbf{Bert4RE + (NFR)\_B}} & \vcell{0.51}                  & \vcell{0.30}                  & \vcell{0.24}                  & \vcell{\textit{0.81}}         & \vcell{\textit{0.74}}         & \vcell{\textit{0.63}}        & \vcell{0.67}                  & \vcell{0.70}                  & \vcell{0.68}                  & \vcell{0.61}                  & \vcell{0.75}                  & \vcell{0.67*}                  \\[-\rowheight]
%\rowcolor[rgb]{0.867,0.867,0.867} 
\printcelltop                       & \printcelltop                 & \printcelltop                 & \printcelltop                 & \printcelltop                 & \printcelltop                 & \printcelltop                 & \printcelltop                 & \printcelltop                 & \printcelltop                 & \printcelltop                 & \printcelltop                 & \printcelltop                  \\
%\rowcolor[rgb]{0.867,0.867,0.867} 
\vcell{\textbf{Bert4RE + (NFR)\_C}} & \vcell{\textbf{0.52}}         & \vcell{\textbf{0.43}}         & \vcell{\textbf{0.46}}         & \vcell{\textbf{0.62}}         & \vcell{\textbf{0.65}}         & \vcell{\textbf{0.63}}         & \vcell{\textbf{\uline{0.72}}} & \vcell{\textbf{\uline{0.73}}} & \vcell{\textbf{\uline{0.72}}} & \vcell{\textbf{0.68}}         & \vcell{\textbf{0.41}}         & \vcell{\textbf{0.43}}          \\[-\rowheight]
%\rowcolor[rgb]{0.867,0.867,0.867} 
\printcelltop                       & \printcelltop                 & \printcelltop                 & \printcelltop                 & \printcelltop                 & \printcelltop                 & \printcelltop                 & \printcelltop                 & \printcelltop                 & \printcelltop                 & \printcelltop                 & \printcelltop                 & \printcelltop                  \\
%\rowcolor[rgb]{0.867,0.867,0.867} 
\vcell{\textbf{Bert4RE + (NFR)\_D}} & \vcell{\textbf{0.54}}         & \vcell{\textbf{0.42}}         & \vcell{\textbf{0.45}}         & \vcell{\textit{0.56}}         & \vcell{\textit{0.70}}         & \vcell{\textit{0.61}}        & \vcell{0.63}                  & \vcell{0.41}                  & \vcell{0.42}                  & \vcell{\textbf{0.60}}         & \vcell{\textbf{0.46}}         & \vcell{\textbf{0.51}}          \\[-\rowheight]
%\rowcolor[rgb]{0.867,0.867,0.867} 
\printcelltop                       & \printcelltop                 & \printcelltop                 & \printcelltop                 & \printcelltop                 & \printcelltop                 & \printcelltop                 & \printcelltop                 & \printcelltop                 & \printcelltop                 & \printcelltop                 & \printcelltop                 & \printcelltop                  \\
%\rowcolor[rgb]{0.867,0.867,0.867} 
\vcell{\textbf{Bert4RE + (NFR)\_E}} & \vcell{\textit{0.53}}         & \vcell{\textit{0.73}}         & \vcell{\textit{0.62}}        & \vcell{\textit{0.54}}         & \vcell{\textit{0.73}}         & \vcell{\textit{0.62}}        & \vcell{0.63}                  & \vcell{0.40}                  & \vcell{0.41}                  & \vcell{0.61}                  & \vcell{0.78}                  & \vcell{\textit{0.69}}                  \\[-\rowheight]
%\rowcolor[rgb]{0.867,0.867,0.867} 
\printcelltop                       & \printcelltop                 & \printcelltop                 & \printcelltop                 & \printcelltop                 & \printcelltop                 & \printcelltop                 & \printcelltop                 & \printcelltop                 & \printcelltop                 & \printcelltop                 & \printcelltop                 & \printcelltop                  \\
\hline
\vcell{\textbf{SObert + (NFR)\_A}}                                    & \vcell{\textit{0.53}}         & \vcell{\textit{0.73}}         & \vcell{\textit{0.62}}        & \vcell{\textit{0.54}}         & \vcell{\textit{0.73}}         & \vcell{\textit{0.62}}        & \vcell{\textit{0.56}}         & \vcell{\textit{0.75}}         & \vcell{\textit{0.64}}        & \vcell{0.61}                  & \vcell{0.78}                  & \vcell{\textit{0.69}}                  \\[-\rowheight]
\printcelltop                                                         & \printcelltop                 & \printcelltop                 & \printcelltop                 & \printcelltop                 & \printcelltop                 & \printcelltop                 & \printcelltop                 & \printcelltop                 & \printcelltop                 & \printcelltop                 & \printcelltop                 & \printcelltop                  \\
\vcell{\textbf{SObert + (NFR)\_B}}                                    & \vcell{\textbf{0.55}}         & \vcell{\textbf{0.51}}         & \vcell{\textbf{0.53}}         & \vcell{\textit{0.81}}         & \vcell{\textit{0.74}}         & \vcell{\textit{0.63}}                 & \vcell{\textit{0.65}}         & \vcell{\textit{0.73}}         & \vcell{\textit{0.67}}         & \vcell{0.61}                  & \vcell{0.78}                  & \vcell{\textit{0.68}}                  \\[-\rowheight]
\printcelltop                                                         & \printcelltop                 & \printcelltop                 & \printcelltop                 & \printcelltop                 & \printcelltop                 & \printcelltop                 & \printcelltop                 & \printcelltop                 & \printcelltop                 & \printcelltop                 & \printcelltop                 & \printcelltop                  \\
\vcell{\textbf{SObert + (NFR)\_C}}                                    & \vcell{0.51}                  & \vcell{0.32}                  & \vcell{0.30}                  & \vcell{\textbf{0.66}}         & \vcell{\textbf{0.53}}         & \vcell{\textbf{0.56}}         & \vcell{\textit{0.71}}         & \vcell{\textit{0.74}}         & \vcell{\textit{0.71}}         & \vcell{\textbf{0.61}}         & \vcell{\textbf{0.55}}         & \vcell{\textbf{0.58}}          \\[-\rowheight]
\printcelltop                                                         & \printcelltop                 & \printcelltop                 & \printcelltop                 & \printcelltop                 & \printcelltop                 & \printcelltop                 & \printcelltop                 & \printcelltop                 & \printcelltop                 & \printcelltop                 & \printcelltop                 & \printcelltop                  \\
\vcell{\textbf{SObert + (NFR)\_E}}                                    & \vcell{0.54}                  & \vcell{0.45}                  & \vcell{0.48}                  & \vcell{\textit{0.58}}         & \vcell{\textit{0.69}}         & \vcell{\textit{0.61}}        & \vcell{\textbf{0.68}}         & \vcell{\textbf{0.58}}         & \vcell{\textbf{0.61}}         & \vcell{0.61}                  & \vcell{0.76}                  & \vcell{0.67}                  \\[-\rowheight]
\printcelltop                                                         & \printcelltop                 & \printcelltop                 & \printcelltop                 & \printcelltop                 & \printcelltop                 & \printcelltop                 & \printcelltop                 & \printcelltop                 & \printcelltop                 & \printcelltop                 & \printcelltop                 & \printcelltop                  \\
\vcell{\textbf{SObert + (NFR)\_D}}                                    & \vcell{\textit{0.53}}         & \vcell{\textit{0.70}}         & \vcell{\textit{0.60}}        & \vcell{\textit{0.63}}         & \vcell{\textit{0.73}}         & \vcell{\textit{0.63}}        & \vcell{0.68}                  & \vcell{0.57}                  & \vcell{0.60}                  & \vcell{0.66}                  & \vcell{0.77}                  & \vcell{0.69}                   \\[-\rowheight]
\printcelltop                                                         & \printcelltop                 & \printcelltop                 & \printcelltop                 & \printcelltop                 & \printcelltop                 & \printcelltop                 & \printcelltop                 & \printcelltop                 & \printcelltop                 & \printcelltop                 & \printcelltop                 & \printcelltop                  \\
\bottomrule
\end{tabular}
}
\end{table}
