# Supplementary material for: Zero-Shot Learning for Requirements Classification: An Exploratory Study
Source: arXiv:2302.04723 source file (2023-03-15)
Supplement: Supplementary file 3 [file SUPPLEMENTARY-resultsFRvsNFR.tex]

\begin{table}
\centering
\scriptsize

\setlength{\extrarowheight}{0pt}
\addtolength{\extrarowheight}{\aboverulesep}
\addtolength{\extrarowheight}{\belowrulesep}
\setlength{\aboverulesep}{0pt}
\setlength{\belowrulesep}{0pt}

\caption{Overall classification results for \textit{Task FR/NFR} for each ZSL Classifier, which is a combination of a specific LM and a specific label configuration. Bold values indicate the best results for a specific ZSL classifier; underlined values indicate the overall best performance across all the classifiers; values in italics indicate a possibly misleading performance, related to the imbalance of F1 between classes.}
\label{tab:resultsFRvsNFR}
\begin{tabular}{llll} 
\toprule
\textbf{ZSL Classifier}                                    & \textbf{wP}      & \textbf{wR}       & \textbf{wF1}          \\ 
\hline
%\rowcolor[rgb]{0.867,0.867,0.867} 

Sbert + FR\_A            & 0.52                  & 0.43                  & 0.35                   \\
%\rowcolor[rgb]{0.867,0.867,0.867} 

Sbert + FR\_B            & 0.60                  & 0.46                  & 0.37                   \\
%\rowcolor[rgb]{0.867,0.867,0.867} 

Sbert + FR\_C            & 0.64                  & 0.48                  & 0.40                   \\
%\rowcolor[rgb]{0.867,0.867,0.867} 

Sbert + FR\_D            & 0.54                  & 0.55                  & 0.54                   \\
%\rowcolor[rgb]{0.867,0.867,0.867} 

\textbf{Sbert + FR\_E}   & \textbf{\uline{0.71}} & \textbf{\uline{0.66}} & \textbf{\uline{0.66}}  \\
%\rowcolor[rgb]{0.867,0.867,0.867} 

Sbert + FR\_F            & 0.69                  & 0.64                  & 0.64                   \\
\hline
AllMini +  FR\_A                                           & 0.56                  & 0.55                  & 0.55                   \\
AllMini +  FR\_B                                           & 0.53                  & 0.48                  & 0.46                   \\
AllMini +  FR\_C                                           & 0.54                  & 0.45                  & 0.39                   \\
\textbf{AllMini + FR\_D}                                   & \textbf{0.63}         & \textbf{0.59}         & \textbf{0.59}          \\
AllMini +  FR\_E                                           & 0.60                  & 0.53                  & 0.51                   \\
AllMini +  FR\_F                                           & 0.66                  & 0.56                  & 0.53                   \\
\hline
%\rowcolor[rgb]{0.867,0.867,0.867} 

Bert4RE +  FR\_A         & 0.35                  & 0.59                  & \textit{0.44}         \\
%\rowcolor[rgb]{0.867,0.867,0.867} 
Bert4RE +  FR\_B         & 0.52                  & 0.56                  & 0.51                   \\
%\rowcolor[rgb]{0.867,0.867,0.867} 
\textbf{Bert4RE + FR\_C} & \textbf{0.58}         & \textbf{0.56}         & \textbf{0.57}          \\
%\rowcolor[rgb]{0.867,0.867,0.867} 
Bert4RE + FR\_D          & 0.59                  & 0.56                  & 0.56                   \\
%\rowcolor[rgb]{0.867,0.867,0.867} 
Bert4RE +  FR\_E         & 0.59                  & 0.52                  & 0.51                   \\
%\rowcolor[rgb]{0.867,0.867,0.867} 
Bert4RE +  FR\_F         & 0.57                  & 0.47                  & 0.42                   \\
\hline
SObert +  FR\_A                                            & 0.35                  & 0.59                  & \textit{0.44}         \\
SObert +  FR\_B                                            & 0.55                  & 0.59                  & 0.51                   \\
\textbf{SObert + FR\_C}                                    & \textbf{0.58}         & \textbf{0.59}         & \textbf{0.58}          \\
SObert +  FR\_D                                            & 0.53                  & 0.58                  & 0.48                   \\
SObert +  FR\_E                                            & 0.60                  & 0.56                  & 0.56                   \\
SObert +  FR\_F                                            & 0.60                  & 0.55                  & 0.54                   \\
\bottomrule
\end{tabular}
\end{table}
