# Supplementary material for: Zero-Shot Learning for Requirements Classification: An Exploratory Study
Source: arXiv:2302.04723 source file (2023-03-15)
Supplement: Supplementary file 4 [file NFRbinLabels.tex]

\begin{table}
\centering
\caption{Label configurations for the remaining NFR classes for Task NFR, binary classification case (continued to table for Table \ref{tab:labelsNFRbinary}).}
  \resizebox{1\textwidth}{!}{
 \label{tab:appendixNFRbinLabels}
\begin{tabular}{llll} 
\toprule
\vcell{\textbf{Label Abbr.}}            & \vcell{\textbf{Label Configuration}}                                                                         & \vcell{\textbf{NFR Label}}                                                                                                                                                                                                                                                                                                                                                                                                            & \vcell{\textbf{"Other" Label}}                                                                                                                                                                                                                       \\[-\rowheight]
\printcelltop                           & \printcelltop                                                                                                & \printcelltop                                                                                                                                                                                                                                                                                                                                                                                                                         & \printcelltop                                                                                                                                                                                                                                        \\ 
\hline
\vcell{\textbf{\textit{Performance}}}   & \vcell{}                                                                                                     & \vcell{}                                                                                                                                                                                                                                                                                                                                                                                                                              & \vcell{}                                                                                                                                                                                                                                             \\[-\rowheight]
\printcelltop                           & \printcelltop                                                                                                & \printcelltop                                                                                                                                                                                                                                                                                                                                                                                                                         & \printcelltop                                                                                                                                                                                                                                        \\
\vcell{\textbf{\textit{PE\_A}}} & \vcell{Original 1}                                                                                           & \vcell{"performance"}                                                                                                                                                                                                                                                                                                                                                                                                                 & \vcell{"not about performance"}                                                                                                                                                                                                                      \\[-\rowheight]
\printcelltop                           & \printcelltop                                                                                                & \printcelltop                                                                                                                                                                                                                                                                                                                                                                                                                         & \printcelltop                                                                                                                                                                                                                                        \\
\vcell{\textbf{\textit{PE\_B}}} & \vcell{Expert curated}                                                                                       & \vcell{"periodic execution or efficacy performance"}                                                                                                                                                                                                                                                                                                                                                                                  & \vcell{"not about periodic execution or efficacy performance"}                                                                                                                                                                                       \\[-\rowheight]
\printcelltop                           & \printcelltop                                                                                                & \printcelltop                                                                                                                                                                                                                                                                                                                                                                                                                         & \printcelltop                                                                                                                                                                                                                                        \\
\vcell{\textbf{\textit{PE\_C}}} & \vcell{\begin{tabular}[b]{@{}l@{}}Word Embedding \\(selected from top 20 words)\end{tabular}}                & \vcell{\begin{tabular}[b]{@{}l@{}}"throughput, reliability, scalability, responsiveness, efficiency, \\workload, benchmark, latency, speed, improvement, or accuracy"\end{tabular}}                                                                                                                                                                                                                                                   & \vcell{\begin{tabular}[b]{@{}l@{}}"not about throughput, reliability, scalability, responsiveness,\\~efficiency, workload, benchmark, latency, speed, improvement,\\~or accuracy"\end{tabular}}                                                      \\[-\rowheight]
\printcelltop                           & \printcelltop                                                                                                & \printcelltop                                                                                                                                                                                                                                                                                                                                                                                                                         & \printcelltop                                                                                                                                                                                                                                        \\
\vcell{\textbf{\textit{PE\_D}}} & \vcell{\begin{tabular}[b]{@{}l@{}}Word Embedding \\(selected from top 20 words) \\+ Original 2\end{tabular}} & \vcell{\begin{tabular}[b]{@{}l@{}}"throughput, reliability, scalability, responsiveness, efficiency,\\~workload, benchmark, latency, speed, improvement, or accuracy"\end{tabular}}                                                                                                                                                                                                                                                   & \vcell{\begin{tabular}[b]{@{}l@{}}"usability, security, operational, look \& feel, legal, fault \& tolerance,\\~maintainability, scalability, availability, or portability"\end{tabular}}                                                            \\[-\rowheight]
\printcelltop                           & \printcelltop                                                                                                & \printcelltop                                                                                                                                                                                                                                                                                                                                                                                                                         & \printcelltop                                                                                                                                                                                                                                        \\
\vcell{\textbf{\textit{PE\_E}}} & \vcell{\begin{tabular}[b]{@{}l@{}}Word Embedding \\(selected from top 50 words) \\+ Original 2\end{tabular}} & \vcell{\begin{tabular}[b]{@{}l@{}}"throughput, reliability, scalability, responsiveness, efficiency, \\workload, benchmark, latency, speed, improvement, accuracy,\\~achieve, tuning, bottleneck, better, high, optimize, effectiveness, \\low, enhances, reducing, incresaed, quality, faster, or degrades"\end{tabular}}                                                                                                            & \vcell{\begin{tabular}[b]{@{}l@{}}"usability, security, operational, look \& feel, legal, fault \& tolerance, \\maintainability, scalability, availability, or portability"\end{tabular}}                                                            \\[-\rowheight]
\printcelltop                           & \printcelltop                                                                                                & \printcelltop                                                                                                                                                                                                                                                                                                                                                                                                                         & \printcelltop                                                                                                                                                                                                                                        \\ 
\hline
\vcell{\textbf{\textit{Operational}}}   & \vcell{}                                                                                                     & \vcell{}                                                                                                                                                                                                                                                                                                                                                                                                                              & \vcell{}                                                                                                                                                                                                                                             \\[-\rowheight]
\printcelltop                           & \printcelltop                                                                                                & \printcelltop                                                                                                                                                                                                                                                                                                                                                                                                                         & \printcelltop                                                                                                                                                                                                                                        \\
\vcell{\textbf{\textit{O\_A}}}  & \vcell{Original 1}                                                                                           & \vcell{"operational"}                                                                                                                                                                                                                                                                                                                                                                                                                 & \vcell{"not about operational"}                                                                                                                                                                                                                      \\[-\rowheight]
\printcelltop                           & \printcelltop                                                                                                & \printcelltop                                                                                                                                                                                                                                                                                                                                                                                                                         & \printcelltop                                                                                                                                                                                                                                        \\
\vcell{\textbf{\textit{O\_B}}}  & \vcell{Expert curated}                                                                                       & \vcell{"working, running, connecting, interfacing, or operative environment"}                                                                                                                                                                                                                                                                                                                                                         & \vcell{\begin{tabular}[b]{@{}l@{}}"not about working, running, connecting, interfacing, \\or operative environment"\end{tabular}}                                                                                                                    \\[-\rowheight]
\printcelltop                           & \printcelltop                                                                                                & \printcelltop                                                                                                                                                                                                                                                                                                                                                                                                                         & \printcelltop                                                                                                                                                                                                                                        \\
\vcell{\textbf{\textit{O\_C}}}  & \vcell{\begin{tabular}[b]{@{}l@{}}Word Embedding\\(selected from top 20 words)\end{tabular}}                 & \vcell{"environmental, organizational, coordination, systemic, or logistics"}                                                                                                                                                                                                                                                                                                                                                         & \vcell{\begin{tabular}[b]{@{}l@{}}"not about environmental, organizational, coordination, \\systemic, or logistics"\end{tabular}}                                                                                                                    \\[-\rowheight]
\printcelltop                           & \printcelltop                                                                                                & \printcelltop                                                                                                                                                                                                                                                                                                                                                                                                                         & \printcelltop                                                                                                                                                                                                                                        \\
\vcell{\textbf{\textit{O\_D}}}  & \vcell{\begin{tabular}[b]{@{}l@{}}Word Embedding \\(selected from top 20 words) \\+ Original 2\end{tabular}} & \vcell{"environmental, organizational, coordination, systemic, or logistics"}                                                                                                                                                                                                                                                                                                                                                         & \vcell{\begin{tabular}[b]{@{}l@{}}"usability, security, performance, look \& feel, legal, fault \& tolerance, \\maintainability, scalability, availability, or portability"\end{tabular}}                                                            \\[-\rowheight]
\printcelltop                           & \printcelltop                                                                                                & \printcelltop                                                                                                                                                                                                                                                                                                                                                                                                                         & \printcelltop                                                                                                                                                                                                                                        \\
\vcell{\textbf{\textit{O\_E}}}  & \vcell{\begin{tabular}[b]{@{}l@{}}Word Embedding \\(selected from top 50 words)\\~+ Original 2\end{tabular}} & \vcell{\begin{tabular}[b]{@{}l@{}}"environmental, organizational, coordination, systemic, logistics,\\~coordination, or automation"\end{tabular}}                                                                                                                                                                                                                                                                                     & \vcell{\begin{tabular}[b]{@{}l@{}}"usability, security, performance, look \& feel, legal, fault \& tolerance, \\maintainability, scalability, availability, or portability"\end{tabular}}                                                            \\[-\rowheight]
\printcelltop                           & \printcelltop                                                                                                & \printcelltop                                                                                                                                                                                                                                                                                                                                                                                                                         & \printcelltop                                                                                                                                                                                                                                        \\ 
\hline
\vcell{\textbf{\textit{Look \& feel}}}  & \vcell{}                                                                                                     & \vcell{}                                                                                                                                                                                                                                                                                                                                                                                                                              & \vcell{}                                                                                                                                                                                                                                             \\[-\rowheight]
\printcelltop                           & \printcelltop                                                                                                & \printcelltop                                                                                                                                                                                                                                                                                                                                                                                                                         & \printcelltop                                                                                                                                                                                                                                        \\
\vcell{\textbf{\textit{LF\_A}}} & \vcell{Original 1}                                                                                           & \vcell{"Look  feel"}                                                                                                                                                                                                                                                                                                                                                                                                                  & \vcell{"not about Look  feel"}                                                                                                                                                                                                                       \\[-\rowheight]
\printcelltop                           & \printcelltop                                                                                                & \printcelltop                                                                                                                                                                                                                                                                                                                                                                                                                         & \printcelltop                                                                                                                                                                                                                                        \\
\vcell{\textbf{\textit{LF\_B}}} & \vcell{Expert curated}                                                                                       & \vcell{"appearance, interface, look  feel"}                                                                                                                                                                                                                                                                                                                                                                                           & \vcell{"not about appearance, interface, look  feel"}                                                                                                                                                                                                \\[-\rowheight]
\printcelltop                           & \printcelltop                                                                                                & \printcelltop                                                                                                                                                                                                                                                                                                                                                                                                                         & \printcelltop                                                                                                                                                                                                                                        \\
\vcell{\textbf{\textit{LF\_C}}} & \vcell{\begin{tabular}[b]{@{}l@{}}Word Embedding\\(selected from top 20 words)\end{tabular}}                 & \vcell{\begin{tabular}[b]{@{}l@{}}"graphical, gui, ui, widget, interaction, habit, prefer, comfortable, friendly, \\feeling, experience, or familiar"\end{tabular}}                                                                                                                                                                                                                                                                   & \vcell{\begin{tabular}[b]{@{}l@{}}" not about graphical, gui, ui, widget, interaction, habit, prefer, \\comfortable, friendly, feeling, experience, or familiar"\end{tabular}}                                                                       \\[-\rowheight]
\printcelltop                           & \printcelltop                                                                                                & \printcelltop                                                                                                                                                                                                                                                                                                                                                                                                                         & \printcelltop                                                                                                                                                                                                                                        \\
\vcell{\textbf{\textit{LF\_D}}} & \vcell{\begin{tabular}[b]{@{}l@{}}Word Embedding\\(selected from top 20 words) \\+ Original 2\end{tabular}}  & \vcell{\begin{tabular}[b]{@{}l@{}}"graphical, gui, ui, widget, interaction, habit, prefer, comfortable, friendly,\\~feeling, experience, or familiar"\end{tabular}}                                                                                                                                                                                                                                                                   & \vcell{\begin{tabular}[b]{@{}l@{}}"usability, security, operational, performance, fault \& tolerance,\\~legal, maintainability, scalability, availability, or portability"\end{tabular}}                                                             \\[-\rowheight]
\printcelltop                           & \printcelltop                                                                                                & \printcelltop                                                                                                                                                                                                                                                                                                                                                                                                                         & \printcelltop                                                                                                                                                                                                                                        \\
\vcell{\textbf{\textit{LF\_E}}} & \vcell{\begin{tabular}[b]{@{}l@{}}Word Embedding \\(selected from top 50 words) \\+ Original 2\end{tabular}} & \vcell{\begin{tabular}[b]{@{}l@{}}"graphical, gui, ui, widget, interaction, habit, prefer, comfortable, friendly,\\~feeling, experience, familiar, desire, customize, intent, disability, \\or impression"\end{tabular}}                                                                                                                                                                                                              & \vcell{\begin{tabular}[b]{@{}l@{}}"usability, security, operational, performance, fault \& tolerance, \\legal, maintainability, scalability, availability, or portability"\end{tabular}}                                                             \\[-\rowheight]
\printcelltop                           & \printcelltop                                                                                                & \printcelltop                                                                                                                                                                                                                                                                                                                                                                                                                         & \printcelltop                                                                                                                                                                                                                                        \\ 
\hline
\vcell{\textbf{\textit{Legal}}}         & \vcell{}                                                                                                     & \vcell{}                                                                                                                                                                                                                                                                                                                                                                                                                              & \vcell{}                                                                                                                                                                                                                                             \\[-\rowheight]
\printcelltop                           & \printcelltop                                                                                                & \printcelltop                                                                                                                                                                                                                                                                                                                                                                                                                         & \printcelltop                                                                                                                                                                                                                                        \\
\vcell{\textbf{\textit{L\_A}}}  & \vcell{Original 1}                                                                                           & \vcell{"legal"}                                                                                                                                                                                                                                                                                                                                                                                                                       & \vcell{"not about legal"}                                                                                                                                                                                                                            \\[-\rowheight]
\printcelltop                           & \printcelltop                                                                                                & \printcelltop                                                                                                                                                                                                                                                                                                                                                                                                                         & \printcelltop                                                                                                                                                                                                                                        \\
\vcell{\textbf{\textit{L\_B}}}  & \vcell{Expert curated}                                                                                       & \vcell{"legal, law, or rules"}                                                                                                                                                                                                                                                                                                                                                                                                        & \vcell{"not about legal, law, or rules"}                                                                                                                                                                                                             \\[-\rowheight]
\printcelltop                           & \printcelltop                                                                                                & \printcelltop                                                                                                                                                                                                                                                                                                                                                                                                                         & \printcelltop                                                                                                                                                                                                                                        \\
\vcell{\textbf{\textit{L\_C}}}  & \vcell{\begin{tabular}[b]{@{}l@{}}Word Embedding \\(selected from top 20 words)\end{tabular}}                & \vcell{\begin{tabular}[b]{@{}l@{}}"liability, litigation, jurisdiction, regulation, copyright, legislation, \\enforcement, governmental, directive, civil, right, patentability,\\~claim, violate, infringement, or counsel"\end{tabular}}                                                                                                                                                                                            & \vcell{\begin{tabular}[b]{@{}l@{}}"not about liability, litigation, jurisdiction, regulation, copyright,\\~legislation, enforcement, governmental, directive,civil, right,\\~patentability, claim, violate, infringement, or counsel"\end{tabular}}  \\[-\rowheight]
\printcelltop                           & \printcelltop                                                                                                & \printcelltop                                                                                                                                                                                                                                                                                                                                                                                                                         & \printcelltop                                                                                                                                                                                                                                        \\
\vcell{\textbf{\textit{L\_D}}}  & \vcell{\begin{tabular}[b]{@{}l@{}}Word Embedding \\(selected from top 20 words) \\+ Original 2\end{tabular}} & \vcell{\begin{tabular}[b]{@{}l@{}}"liability, litigation, jurisdiction, regulation, copyright, legislation,\\enforcement, governmental, directive,civil, right, patentability,\\~claim, violate, infringement, or counsel"\end{tabular}}                                                                                                                                                                                              & \vcell{\begin{tabular}[b]{@{}l@{}}"usability, security, operational, performance, look \& feel,\\~fault \& tolerance, maintainability, scalability, availability, \\or portability"\end{tabular}}                                                    \\[-\rowheight]
\printcelltop                           & \printcelltop                                                                                                & \printcelltop                                                                                                                                                                                                                                                                                                                                                                                                                         & \printcelltop                                                                                                                                                                                                                                        \\
\vcell{\textbf{\textit{L\_E}}}  & \vcell{\begin{tabular}[b]{@{}l@{}}Word Embedding \\(selected from top 50 words) \\+ Original 2\end{tabular}} & \vcell{\begin{tabular}[b]{@{}l@{}}"liability, litigation, jurisdiction, regulation, copyright, legislation,\\~enforcement, governmental, directive,civil, right, patentability, \\claim, violate, infringement,~~counsel, holder, dispute, illegal, judicial,\\~ruling, agreement, ownership, comply, authority, law, accountability, \\abuse, intellectual, obligation, invention,~court, ethical, concern, or policy"\end{tabular}} & \vcell{\begin{tabular}[b]{@{}l@{}}"usability, security, operational, performance, look \& feel, \\fault \& tolerance, maintainability, scalability, availability, \\or portability"\end{tabular}}                                                    \\[-\rowheight]
\printcelltop                           & \printcelltop                                                                                                & \printcelltop                                                                                                                                                                                                                                                                                                                                                                                                                         & \printcelltop                                                                                                                                                                                                                                        \\
\bottomrule
\end{tabular}
}
\end{table}

\addtocounter{table}{-1}

\begin{table}
\centering
\caption{Continued }
  \resizebox{1\textwidth}{!}{
\begin{tabular}{llll} 
\toprule
\textbf{Label Abbr.}               & \textit{\textbf{Label Configuration}}                                                                & \textit{\textbf{NFR Label}}                                                                                                                                                                                                                                           & \textit{\textbf{"Other" Label}}                                                                                                                                                                                                                                                  \\ 
\hline
\textbf{\textit{Fault tolerance}}  &                                                                                                      &                                                                                                                                                                                                                                                                       &                                                                                                                                                                                                                                                                                  \\
\textbf{\textit{FT\_A}}    & Original 1                                                                                           & "fault  tolerance"                                                                                                                                                                                                                                                    & "not about fault  tolerance"                                                                                                                                                                                                                                                     \\
\textbf{\textit{FT\_B}}    & Expert curated                                                                                       & "system recovery  fault tolerance"                                                                                                                                                                                                                                    & "not about system recovery  fault tolerance"                                                                                                                                                                                                                                     \\
\textbf{\textit{FT\_C}}    & \begin{tabular}[c]{@{}l@{}}Word Embedding \\(selected from top 20 words)\end{tabular}                & \begin{tabular}[c]{@{}l@{}}"tolerance, failure, tolerant, byzantine, deadlock, exploiting, \\reliability, isolation, fault, guarantee, or dependable"\end{tabular}                                                                                                    & \begin{tabular}[c]{@{}l@{}}"not about tolerance, failure, tolerant, byzantine, deadlock, exploiting, reliability,\\~isolation, fault, guarantee, dependable, countermeasure, resilience, defensive,\\~corruption, weakness, malfunction, robustness, or stability"\end{tabular}  \\
\textbf{\textit{FT\_D}}    & \begin{tabular}[c]{@{}l@{}}Word Embedding \\(selected from top 20 words) \\+ Original 2\end{tabular} & \begin{tabular}[c]{@{}l@{}}"tolerance, failure, tolerant, byzantine, deadlock, exploiting,\\~reliability, isolation, fault, guarantee, or dependable"\end{tabular}                                                                                                    & \begin{tabular}[c]{@{}l@{}}"usability, security, operational, performance, look \& feel, legal, maintainability, \\scalability, availability, or portability"\end{tabular}                                                                                                       \\
\textbf{\textit{FT\_E}}    & \begin{tabular}[c]{@{}l@{}}Word Embedding \\(selected from top 50 words) \\+ Original 2\end{tabular} & \begin{tabular}[c]{@{}l@{}}"tolerance, failure, tolerant, byzantine, deadlock, exploiting,\\~reliability, isolation, fault, guarantee, dependable, countermeasure, \\resilience, defensive, corruption, weakness, malfunction, robustness, or stability"\end{tabular} & \begin{tabular}[c]{@{}l@{}}"usability, security, operational, performance, look \& feel, legal, maintainability,\\~scalability, availability, or portability"\end{tabular}                                                                                                       \\ 
\hline
\textbf{\textit{Maintainability~}} &                                                                                                      &                                                                                                                                                                                                                                                                       &                                                                                                                                                                                                                                                                                  \\
\textbf{\textit{MN\_A}}    & Original 1                                                                                           & "maintainability"                                                                                                                                                                                                                                                     & "not about maintainability"                                                                                                                                                                                                                                                      \\
\textbf{\textit{MN\_B}}    & Expert curated                                                                                       & "maintaining, fixing, running or updating"                                                                                                                                                                                                                            & "not about maintaining, fixing, running or updating"                                                                                                                                                                                                                             \\
\textbf{\textit{MN\_C}}    & \begin{tabular}[c]{@{}l@{}}Word Embedding\\(selected from top 20 words)\end{tabular}                 & "adaptability, effectiveness, agility, preventive, or dependability"                                                                                                                                                                                                  & "not about adaptability, effectiveness, agility, preventive, or dependability"                                                                                                                                                                                                   \\
\textbf{\textit{MN\_D}}    & \begin{tabular}[c]{@{}l@{}}Word Embedding \\(selected from top 20 words) \\+ Original 2\end{tabular} & "adaptability, effectiveness, agility, preventive, or dependability"                                                                                                                                                                                                  & \begin{tabular}[c]{@{}l@{}}"usability, security, operational, performance, look \& feel, legal, fault \& tolerance, \\scalability, availability, or portability"\end{tabular}                                                                                                    \\
\textbf{\textit{MN\_E}}    & \begin{tabular}[c]{@{}l@{}}Word Embedding \\(selected from top 50 words) \\+ Original 2\end{tabular} & \begin{tabular}[c]{@{}l@{}}"adaptability, effectiveness, agility, preventive, dependability, \\correcting, reuse, defect, mitigation, validated, resilience, achievable, \\remedy, assessing, or maintaining"\end{tabular}                                            & \begin{tabular}[c]{@{}l@{}}"usability, security, operational, performance, look \& feel, legal, fault \& tolerance, \\scalability, availability, or portability"\end{tabular}                                                                                                    \\ 
\hline
\textbf{\textit{Scalability}}      &                                                                                                      &                                                                                                                                                                                                                                                                       &                                                                                                                                                                                                                                                                                  \\
\textbf{\textit{SC\_A}}    & Original 1                                                                                           & "scalability"                                                                                                                                                                                                                                                         & "not about scalability"                                                                                                                                                                                                                                                          \\
\textbf{\textit{SC\_B}}    & Expert curated                                                                                       & "scalable, increasable or developable"                                                                                                                                                                                                                                & "not about scalable, increasable or developable"                                                                                                                                                                                                                                 \\
\textbf{\textit{SC\_C}}    & \begin{tabular}[c]{@{}l@{}}Word Embedding \\(selected from top 20 words)\end{tabular}                & "flexibility, workload, efficiency, or optimize"                                                                                                                                                                                                                      & "not about flexibility, workload, efficiency, or optimize"                                                                                                                                                                                                                       \\
\textbf{\textit{SC\_D}}    & \begin{tabular}[c]{@{}l@{}}Word Embedding \\(selected from top 20 words) \\+ Original 2\end{tabular} & "flexibility, workload, efficiency, or optimize"                                                                                                                                                                                                                      & \begin{tabular}[c]{@{}l@{}}"usability, security, operational, performance, look \& feel, legal, fault \& tolerance, \\maintainability, availability, or portability"\end{tabular}                                                                                                \\
\textbf{\textit{SC\_E}}    & \begin{tabular}[c]{@{}l@{}}Word Embedding \\(selected from top 50 words) \\+ Original 2\end{tabular} & \begin{tabular}[c]{@{}l@{}}"flexibility, workload, efficiency, optimize, caching, improvement,\\~robust, overhead, adaptability, scalable, or increased"\end{tabular}                                                                                                 & \begin{tabular}[c]{@{}l@{}}"usability, security, operational, performance, look \& feel, legal, fault \& tolerance,\\~maintainability, availability, or portability"\end{tabular}                                                                                                \\ 
\hline
\textbf{\textit{Availability~}}    &                                                                                                      &                                                                                                                                                                                                                                                                       &                                                                                                                                                                                                                                                                                  \\
\textbf{\textit{A\_A}}     & Original 1                                                                                           & "availability"                                                                                                                                                                                                                                                        & "not about availability"                                                                                                                                                                                                                                                         \\
\textbf{\textit{A\_B}}     & Expert curated                                                                                       & "avaliable or timely achievable"                                                                                                                                                                                                                                      & "not about avaliable or timely achievable"                                                                                                                                                                                                                                       \\
\textbf{\textit{A\_C}}     & \begin{tabular}[c]{@{}l@{}}Word Embedding \\(selected from top 20 words)\end{tabular}                & "reliability, dependability, resilience"                                                                                                                                                                                                                              & "not about reliability, dependability, resilience"                                                                                                                                                                                                                               \\
\textbf{\textit{A\_D}}     & \begin{tabular}[c]{@{}l@{}}Word Embedding \\(selected from top 20 words)\\+ Original 2\end{tabular}  & "reliability, dependability, resilience"                                                                                                                                                                                                                              & \begin{tabular}[c]{@{}l@{}}"usability, security, operational, performance, look \& feel, legal, fault \& tolerance,\\~maintainability, scalability, or portability"\end{tabular}                                                                                                 \\
\textbf{\textit{A\_E}}     & \begin{tabular}[c]{@{}l@{}}Word Embedding \\(selected from top 50 words) \\+ Original 2\end{tabular} & \begin{tabular}[c]{@{}l@{}}"reliability, dependability, resilience, flexibility, accountability, \\ensur, disruption, timely, or standby"\end{tabular}                                                                                                                & \begin{tabular}[c]{@{}l@{}}"usability, security, operational, performance, look \& feel, legal, fault~~\& tolerance,\\~maintainability, scalability, or portability"\end{tabular}                                                                                                \\
\bottomrule
\end{tabular}
}
\end{table}
