# Supplementary material for: Zero-Shot Learning for Requirements Classification: An Exploratory Study
Source: arXiv:2302.04723 source file (2023-03-15)
Supplement: Supplementary file 5 [file SUPPLEMENTARY-AllNFRmultiLabelResults.tex]

\begin{table}
\centering
\setlength{\extrarowheight}{0pt}
\addtolength{\extrarowheight}{\aboverulesep}
\addtolength{\extrarowheight}{\belowrulesep}
\setlength{\aboverulesep}{0pt}
\setlength{\belowrulesep}{0pt}
\caption{Multi-label classification results for all NFR classes---Top 3 results---369 requirements from PROMISE dataset.}
\label{tab:AllNFRmultiLabelResults}
  \resizebox{1\textwidth}{!}{
\begin{tabular}{l|ccc|ccc|ccc|ccc|ccc} 
\toprule
\multicolumn{1}{c|}{\multirow{2}{*}{\textbf{ZSL Classifier}}} & \multicolumn{3}{c|}{\textbf{US}}                                      & \multicolumn{3}{c|}{\textbf{SE}}                                      & \multicolumn{3}{c|}{\textbf{O}}                                        & \multicolumn{3}{c|}{\textbf{PE}}                                      & \multicolumn{3}{c}{\textbf{LF}}                                        \\ 
\cline{2-16}
\multicolumn{1}{c|}{}                                     & \textbf{P}        & \textbf{R}         & \textbf{F1}        & \textbf{P}        & \textbf{R}         & \textbf{F1}        & \textbf{P}        & \textbf{R}         & \textbf{F1}        & \textbf{P}        & \textbf{R}         & \textbf{F1}        & \textbf{P}        & \textbf{R}         & \textbf{F1}         \\ 
\hline
%\rowcolor[rgb]{0.867,0.867,0.867} 
Sbert + MultiNFR\_A     & 0.74                  & 0.55                  & 0.63                  & \textbf{0.78}         & \textbf{0.71}         & \textbf{0.75}         & 0.56                  & 0.53                  & 0.55                  & 0.73                  & 0.35                  & 0.48                  & 0.64                  & 0.37                  & 0.47                   \\
%\rowcolor[rgb]{0.867,0.867,0.867} 
Sbert + MultiNFR\_B     & \textbf{\uline{0.87}} & \textbf{0.51}         & \textbf{\uline{0.64}} & 0.87                  & 0.62                  & 0.73                  & \textbf{0.71}         & \textbf{0.74}         & \textbf{\uline{0.72}} & \textbf{0.62}         & \textbf{\uline{0.69}} & \textbf{0.65}         & \textbf{0.55}         & \textbf{\uline{0.76}} & \textbf{0.64}          \\
%\rowcolor[rgb]{0.867,0.867,0.867} 
Sbert + MultiNFR\_C     & 0.76                  & 0.39                  & 0.51                  & \textbf{0.80}         & \textbf{0.71}         & \textbf{0.75}         & 0.80                  & 0.39                  & 0.52                  & 0.41                  & 0.81                  & 0.54                  & 0.68                  & 0.55                  & 0.61                   \\
%\rowcolor[rgb]{0.867,0.867,0.867} 
Sbert + MultiNFR\_D     & 0.82                  & 0.40                  & 0.54                  & 0.90                  & 0.58                  & 0.70                  & 0.63                  & 0.73                  & 0.68                  & 0.81                  & 0.46                  & 0.59                  & 0.46                  & 0.58                  & 0.51                   \\
\hline
AllMini + MultiNFR\_A                                     & 0.73                  & 0.45                  & 0.56                  & \textbf{\uline{0.92}} & \textbf{\uline{0.88}} & \textbf{\uline{0.90}} & 0.52                  & 0.90                  & 0.28                  & 0.76                  & 0.46                  & 0.57                  & 1.00                  & 0.32                  & 0.48                   \\
AllMini + MultiNFR\_B                                     & 1.00                  & 0.40                  & 0.57                  & 0.80                  & 0.92                  & 0.86                  & \textbf{\uline{0.78}} & \textbf{0.52}         & \textbf{0.62}         & \textbf{0.70}         & \textbf{0.65}         & \textbf{\uline{0.67}} & \textbf{0.71}         & \textbf{0.63}         & \textbf{\uline{0.67}}  \\
AllMini + MultiNFR\_C                                     & \textbf{0.79}         & \textbf{0.49}         & \textbf{0.61}         & 0.96                  & 0.39                  & 0.56                  & 0.49                  & 0.32                  & 0.39                  & 0.56                  & 0.52                  & 0.54                  & 0.79                  & 0.29                  & 0.42                   \\
AllMini + MultiNFR\_D                                     & 1.00                  & 0.36                  & 0.53                  & 1.00                  & 0.22                  & 0.37                  & 0.32                  & 0.35                  & 0.34                  & 1.00                  & 0.33                  & 0.50                  & 0.75                  & 0.32                  & 0.28                   \\
\hline
%\rowcolor[rgb]{0.867,0.867,0.867} 
Bert4RE + MultiNFR\_A   & 1.00                  & 0.16                  & 0.28                  & 1.00                  & 0.09                  & 0.17                  & 1.00                  & 0.10                  & 0.18                  & \textbf{\uline{1.00}} & \textbf{0.52}         & \textbf{0.68}         & 0.60                  & 0.39                  & 0.48                   \\
%\rowcolor[rgb]{0.867,0.867,0.867} 
Bert4RE + MultiNFR\_B   & \textbf{0.29}         & \textbf{\uline{0.66}} & \textbf{0.40}         & \textit{0.00}           & \textit{0.00}           & \textit{0.00}           & \textbf{0.35}         & \textbf{\uline{0.81}} & \textbf{0.49}         & 0.83                  & 0.09                  & 0.17                  & 0.63                  & 0.58                  & 0.60                   \\
%\rowcolor[rgb]{0.867,0.867,0.867} 
Bert4RE + MultiNFR\_C   & 1.00                  & 0.06                  & 0.11                  & \textbf{0.50}         & \textbf{0.27}         & \textbf{0.35}         & 0.25                  & 0.71                  & 0.37                  & 1.00                  & 0.13                  & 0.23                  & 0.33                  & 0.37                  & 0.35                   \\
%\rowcolor[rgb]{0.867,0.867,0.867} 
Bert4RE + MultiNFR\_D   & 1.00                  & 0.03                  & 0.06                  & \textit{0.00}           & \textit{0.00}           & \textit{0.00}            & 0.22                  & 0.89                  & 0.35                  & 0.30                  & 0.19                  & 0.23                  & \textbf{\uline{1.00}} & \textbf{0.45}         & \textbf{0.62}          \\
\hline
SObert + MultiNFR\_A                                      & \textit{0.00}           & \textit{0.00}           & \textit{0.00}            & \textit{0.00}           & \textit{0.00}           & \textit{0.00}            & 1.00                  & 0.06                  & 0.12                  & 1.00                  & 0.04                  & 0.07                  & \textit{0.00}           & \textit{0.00}           & \textit{0.00}             \\
SObert + MultiNFR\_B                                      & 0.28                  & 0.85                  & 0.43                  & \textit{0.00}           & \textit{0.00}           & \textit{0.00}             & \textbf{0.62}         & \textbf{0.76}         & \textbf{0.68}         & \textbf{0.40}         & \textbf{0.19}         & \textbf{0.25}         & \textbf{0.93}         & \textbf{0.34}         & \textbf{0.50}          \\
SObert + MultiNFR\_C                                      & \textbf{0.54}         & \textbf{0.63}         & \textbf{0.58}         & \textbf{0.64}         & \textbf{0.32}         & \textbf{0.42}         & 0.60                  & 0.65                  & 0.62                  & \textit{0.00}           & \textit{0.00}           & \textit{0.00}             & \textit{0.00}           & \textit{0.00}           & \textit{0.00}            \\
SObert + MultiNFR\_E                                      & \textit{0.00}           & \textit{0.00}           & \textit{0.00}            & \textit{0.00}           & \textit{0.00}           & \textit{0.00}            & 0.42                  & 0.77                  & 0.55                  & \textit{0.00}           & \textit{0.00}           & \textit{0.00}            & \textit{0.00}           & \textit{0.00}           & \textit{0.00}             \\
\bottomrule
\toprule
\toprule
\multicolumn{1}{c|}{\multirow{2}{*}{\textbf{ZSL classifier}}} & \multicolumn{3}{c|}{\textbf{SC}}                                      & \multicolumn{3}{c|}{\textbf{A}}                                       & \multicolumn{3}{c|}{\textbf{MN}}                                      & \multicolumn{3}{c|}{\textbf{L}}                                       & \multicolumn{3}{c}{\textbf{FT}}                                        \\ 
\cline{2-16}
\multicolumn{1}{c|}{}                                         & \textbf{P}        & \textbf{R}         & \textbf{F1}        & \textbf{P}        & \textbf{R}         & \textbf{F1}        & \textbf{P}        & \textbf{R}         & \textbf{F1}        & \textbf{P}        & \textbf{R}         & \textbf{F1}        & \textbf{P}        & \textbf{R}         & \textbf{F1}         \\ 
\hline
%\rowcolor[rgb]{0.867,0.867,0.867} 
Sbert + MultiNFR\_A         & \textbf{0.53}         & \textbf{0.76}         & \textbf{0.63}         & 0.41                  & 0.33                  & 0.37                  & 0.16                  & 0.59                  & 0.25                  & 0.50                  & 0.31                  & 0.38                  & 0.22                  & 0.70                  & 0.33                   \\
%\rowcolor[rgb]{0.867,0.867,0.867} 
Sbert + MultiNFR\_B         & 0.55                  & 0.29                  & 0.38                  & 0.83                  & 0.24                  & 0.37                  & \textbf{0.42}         & \textbf{\uline{0.94}} & \textbf{0.58}         & \textbf{\uline{1.00}} & \textbf{0.31}         & \textbf{0.47}         & 0.20                  & 0.90                  & 0.32                   \\
%\rowcolor[rgb]{0.867,0.867,0.867} 
Sbert + MultiNFR\_C         & 0.36                  & 0.81                  & 0.50                  & 0.50                  & 0.14                  & 0.22                  & 0.36                  & 0.47                  & 0.41                  & 0.38                  & 0.38                  & 0.38                  & 0.21                  & 0.40                  & 0.28                   \\
%\rowcolor[rgb]{0.867,0.867,0.867} 
Sbert + MultiNFR\_D         & 0.24                  & 0.81                  & 0.38                  & \textbf{0.33}         & \textbf{0.76}         & \textbf{0.46}         & 0.57                  & 0.47                  & 0.52                  & 0.42                  & 0.23                  & 0.30                  & \textbf{0.67}         & \textbf{0.40}         & \textbf{0.50}          \\
\hline
AllMini + MultiNFR\_A                                         & \textbf{0.45}         & \textbf{0.81}         & \textbf{0.58}         & 0.31                  & 1.00                  & 0.48                  & 0.58                  & 0.65                  & 0.61                  & \textbf{0.43}         & \textbf{\uline{0.77}} & \textbf{\uline{0.56}} & 0.14                  & 0.70                  & 0.23                   \\
AllMini + MultiNFR\_B                                         & 0.57                  & 0.57                  & 0.57                  & \textbf{0.54}         & \textbf{0.95}         & \textbf{0.69}         & \textbf{0.62}         & \textbf{0.76}         & \textbf{0.68}         & 0.35                  & 1.00                  & 0.52                  & 0.24                  & 0.60                  & 0.34                   \\
AllMini + MultiNFR\_C                                         & 0.35                  & 0.81                  & 0.49                  & 0.15                  & 0.81                  & 0.26                  & 0.33                  & 0.35                  & 0.34                  & 0.50                  & 0.34                  & 0.52                  & 1.00                  & 0.50                  & 0.67                   \\
AllMini + MultiNFR\_D                                         & 0.22                  & 0.38                  & 0.28                  & 0.30                  & 1.00                  & 0.46                  & 0.09                  & 0.59                  & 0.18                  & 1.00                  & 0.31                  & 0.47                  & \textbf{\uline{1.00}} & \textbf{\uline{0.60}} & \textbf{\uline{0.75}}  \\
\hline
%\rowcolor[rgb]{0.867,0.867,0.867} 
Bert4RE + MultiNFR\_A       & \textbf{\uline{1.00}} & \textbf{0.62}         & \textbf{0.76}         & \textit{0.00}           & \textit{0.00}           & \textit{0.00}                    & 0.06                  & 1.00                  & 0.11                  & \textit{0.00}           & \textit{0.00}           & \textit{0.00}            & \textit{0.00}           & \textit{0.00}           & \textit{0.00}             \\
%\rowcolor[rgb]{0.867,0.867,0.867} 
Bert4RE + MultiNFR\_B       & 1.00                  & 0.05                  & 0.09                  & 0.40                  & 0.57                  & 0.47                  & 1.00                  & 0.12                  & 0.21                 & \textit{0.00}           & \textit{0.00}           & \textit{0.00}            & \textit{0.00}           & \textit{0.00}           & \textit{0.00}             \\
%\rowcolor[rgb]{0.867,0.867,0.867} 
Bert4RE + MultiNFR\_C       & 0.14                  & 0.05                  & 0.07                  & 0.24                  & 0.62                  & 0.35                  & \textbf{0.67}         & \textbf{0.47}         & \textbf{0.55}        & \textit{0.00}           & \textit{0.00}           & \textit{0.00}            & \textbf{0.05}         & \textbf{0.10}         & \textbf{0.07}          \\
%\rowcolor[rgb]{0.867,0.867,0.867} 
Bert4RE + MultiNFR\_D       & 0.24                  & 0.19                  & 0.21                  & \textbf{\uline{1.00}} & \textbf{0.76}         & \textbf{\uline{0.86}} & 0.37                  & 0.65                  & 0.47                  & \textit{0.00}           & \textit{0.00}           & \textit{0.00}            & \textit{0.00}           & \textit{0.00}           & \textit{0.00}             \\
\hline
SObert + MultiNFR\_A                                          & \textit{0.00}           & \textit{0.00}           & \textit{0.00}            & \textit{0.00}           & \textit{0.00}           & \textit{0.00}           & \textbf{\uline{1.00}} & \textbf{\uline{0.94}} & \textbf{\uline{0.97}} & \textit{0.00}           & \textit{0.00}           & \textit{0.00}             & 1.00                  & 1.00                  & 1.00                   \\
SObert + MultiNFR\_B                                          & 0.33                  & 0.71                  & 0.45                  & \textit{0.00}           & \textit{0.00}           & \textit{0.00}            & \textit{0.00}           & \textit{0.00}           & \textit{0.00}            & \textbf{0.50}         & \textbf{0.31}         & \textbf{0.38}        & \textit{0.00}           & \textit{0.00}           & \textit{0.00}            \\
SObert + MultiNFR\_C                                          & 1.00                  & 0.14                  & 0.25                  & 0.20                  & 0.14                  & 0.17                  & 0.06                  & 0.41                  & 0.11                  & 0.02                  & 0.08                  & 0.03                  & \textbf{0.13}         & \textbf{0.20}         & \textbf{0.15}          \\
SObert + MultiNFR\_E                                          & \textbf{\uline{1.00}} & \textbf{\uline{0.95}} & \textbf{\uline{0.98}} & \textbf{0.10}         & \textbf{\uline{0.95}} & \textbf{0.19}         & 0.24                  & 0.53                  & 0.33                  & \textit{0.00}           & \textit{0.00}           & \textit{0.00}           & 0.25                  & 0.10                  & 0.14                   \\
\bottomrule
\end{tabular}
}
\end{table}
