# Supplementary material for: Zero-Shot Learning for Requirements Classification: An Exploratory Study
Source: arXiv:2302.04723 source file (2023-03-15)
Supplement: Supplementary file 6 [file SUPPLEMENTARY-AllNFRmultiResults.tex]

\begin{table}
\centering
\setlength{\extrarowheight}{0pt}
\addtolength{\extrarowheight}{\aboverulesep}
\addtolength{\extrarowheight}{\belowrulesep}
\setlength{\aboverulesep}{0pt}
\setlength{\belowrulesep}{0pt}

\caption{Overall performance results of multi-class classification of all 10 NFR classes in PROMISE dataset (369 requirements) for \textit{Task NFR}. \hl{put in shared material}}
\label{tab:NFRmultiAll}

\resizebox{1\textwidth}{!}{
\begin{tabular}{l|ccc|ccc|ccc|ccc|ccc} 
\toprule
\multicolumn{1}{c|}{\multirow{2}{*}{\textbf{ZSL Classifier}}} & \multicolumn{3}{c|}{\textbf{US}}                                      & \multicolumn{3}{c|}{\textbf{SE}}                                      & \multicolumn{3}{c|}{\textbf{O}}                                       & \multicolumn{3}{c|}{\textbf{PE}}                                      & \multicolumn{3}{c}{\textbf{LF}}                                        \\ 
\cline{2-16}
\multicolumn{1}{c|}{}                                     & \textbf{P}        & \textbf{R}         & \textbf{F1}        & \textbf{P}        & \textbf{R}         & \textbf{F1}        & \textbf{P}        & \textbf{R}         & \textbf{F1}        & \textbf{P}        & \textbf{R}         & \textbf{F1}        & \textbf{P}        & \textbf{R}         & \textbf{F1}         \\ 
\hline
%\rowcolor[rgb]{0.867,0.867,0.867} 
Sbert + MultiNFR\_A     & 0.50                  & 0.21                  & 0.29                  & 0.56                  & 0.44                  & 0.49                  & 0.29                  & 0.24                  & 0.26                  & 0.29                  & 0.07                  & 0.12                  & 0.33                  & 0.13                  & 0.19                   \\
%\rowcolor[rgb]{0.867,0.867,0.867} 
Sbert + MultiNFR\_B     & \textbf{0.64}         & \textbf{0.31}         & \textbf{\uline{0.42}} & \textbf{0.76}         & \textbf{0.38}         & \textbf{0.51}         & \textbf{0.44}         & \textbf{\uline{0.32}} & \textbf{0.37}         & \textbf{0.30}         & \textbf{0.26}         & \textbf{0.28}         & \textbf{0.34}         & \textbf{\uline{0.58}} & \textbf{0.43}          \\
%\rowcolor[rgb]{0.867,0.867,0.867} 
Sbert + MultiNFR\_C     & 0.28                  & 0.07                  & 0.12                  & 0.57                  & 0.44                  & 0.50                  & 0.52                  & 0.18                  & 0.27                  & 0.15                  & 0.31                  & 0.20                  & 0.28                  & 0.18                  & 0.22                   \\
%\rowcolor[rgb]{0.867,0.867,0.867} 
Sbert + MultiNFR\_D     & 0.39                  & 0.10                  & 0.16                  & 0.74                  & 0.30                  & 0.43                  & 3.32                  & 0.32                  & 0.32                  & 0.61                  & 0.20                  & 0.31                  & 0.20                  & 0.29                  & 0.23                   \\
\hline
AllMini + MultiNFR\_A                                     & \textbf{0.48}         & \textbf{0.16}         & \textbf{0.24}         & \textbf{\uline{0.79}} & \textbf{\uline{0.62}} & \textbf{\uline{0.69}} & 0.20                  & 0.06                  & 0.10                  & \textbf{\uline{0.56}} & \textbf{\uline{0.28}} & \textbf{\uline{0.37}} & 1.00                  & 0.13                  & 0.23                   \\
AllMini + MultiNFR\_B                                     & \textbf{\uline{1.00}} & \textbf{0.13}         & \textbf{0.24}         & 0.70                  & 0.67                  & 0.68                  & \textbf{\uline{0.60}} & \textbf{0.29}         & \textbf{\uline{0.39}} & 0.13                  & 0.06                  & 0.08                  & \textbf{\uline{0.51}} & \textbf{0.47}         & \textbf{\uline{0.49}}  \\
AllMini + MultiNFR\_C                                     & 0.28                  & 0.07                  & 0.12                  & 0.88                  & 0.21                  & 0.34                  & 0.18                  & 0.15                  & 0.16                  & 0.29                  & 0.28                  & 0.28                  & 0.22                  & 0.05                  & 0.09                   \\
AllMini + MultiNFR\_D                                     & 1.00                  & 0.01                  & 0.03                  & 1.00                  & 0.02                  & 0.03                  & 0.16                  & 0.19                  & 0.18                  & 1.00                  & 0.02                  & 0.04                  & \textit{0.00}           & \textit{0.00}           & \textit{0.00}            \\
\hline
%\rowcolor[rgb]{0.867,0.867,0.867} 
Bert4RE + MultiNFR\_A   & \textit{0.00}           & \textit{0.00}           & \textit{0.00}           & \textit{0.00}           & \textit{0.00}           & \textit{0.00}           & \textit{0.00}           & \textit{0.00}           & \textit{0.00}           & \textit{0.00}           & \textit{0.00}           & \textit{0.00}           & 0.11                  & 0.18                  & 0.14                   \\
%\rowcolor[rgb]{0.867,0.867,0.867} 
Bert4RE + MultiNFR\_B   & \textbf{0.23}         & \textbf{\uline{0.60}} & \textbf{0.33}         & \textit{0.00}           & \textit{0.00}           & \textit{0.00}           & 0.17                  & 0.39                  & 0.24                  & 0.50                  & 0.02                  & 0.04                  & 0.05                  & 0.03                  & 0.04                   \\
%\rowcolor[rgb]{0.867,0.867,0.867} 
Bert4RE + MultiNFR\_C   & \textit{0.00}           & \textit{0.00}           & \textit{0.00}           & \textbf{0.16}         & \textbf{0.06}         & \textbf{0.09}         & 0.16                  & 0.47                  & 0.23                  & \textit{0.00}                    & \textit{0.00}                    & \textit{0.00}                    & \textbf{0.19}         & \textbf{0.21}         & \textbf{0.20}          \\
%\rowcolor[rgb]{0.867,0.867,0.867} 
Bert4RE + MultiNFR\_D   & \textit{0.00}           & \textit{0.00}           & \textit{0.00}           & \textit{0.00}           & \textit{0.00}           & \textit{0.00}           & \textbf{0.16}         & \textbf{0.73}         & \textbf{0.26}         & \textbf{0.19}         & \textbf{0.13}         & \textbf{0.16}         & \textit{0.00}           & \textit{0.00}           & \textit{0.00}            \\
\hline
SObert + MultiNFR\_A                                      & \textit{0.00}           & \textit{0.00}           & \textit{0.00}           & \textit{0.00}           & \textit{0.00}           & \textit{0.00}           & \textit{0.00}           & \textit{0.00}           & \textit{0.00}           & \textit{0.00}           & \textit{0.00}           & \textit{0.00}           & \textbf{0.10}         & \textbf{0.95}         & \textbf{0.18}          \\
SObert + MultiNFR\_B                                      & \textbf{0.21}         & \textbf{0.81}         & \textbf{0.33}         & \textit{0.00}           & \textit{0.00}           & \textit{0.00}           & 0.16                  & 0.11                  & 0.13                  & \textbf{0.14}         & \textbf{0.06}         & \textbf{0.08}         & 0.50                  & 0.05                  & 0.10                   \\
SObert + MultiNFR\_C                                      & 0.23                  & 0.18                  & 0.20                  & \textbf{0.16}         & \textbf{0.05}         & \textbf{0.07}         & 0.29                  & 0.21                  & 0.24                  & \textit{0.00}           & \textit{0.00}           & \textit{0.00}           & \textit{0.00}           & \textit{0.00}           & \textit{0.00}            \\
SObert + MultiNFR\_E                                      & \textit{0.00}           & \textit{0.00}           & \textit{0.00}           & \textit{0.00}           & \textit{0.00}           & \textit{0.00}           & \textbf{0.21}         & \textbf{0.34}         & \textbf{0.26}         & \textit{0.00}           & \textit{0.00}           & \textit{0.00}           & \textit{0.00}           & \textit{0.00}           & \textit{0.00}            \\
\bottomrule
\toprule
\toprule
\multicolumn{1}{c|}{\multirow{2}{*}{\textbf{ZSL Classifier}}} & \multicolumn{3}{c|}{\textbf{SC}}                                      & \multicolumn{3}{c|}{\textbf{A}}                                       & \multicolumn{3}{c|}{\textbf{MN}}                                      & \multicolumn{3}{c|}{\textbf{L}}                                       & \multicolumn{3}{c}{\textbf{FT}}                                        \\ 
\cline{2-16}
\multicolumn{1}{c|}{}                                     & \textbf{P}        & \textbf{R}         & \textbf{F1}        & \textbf{P}        & \textbf{R}         & \textbf{F1}        & \textbf{P}        & \textbf{R}         & \textbf{F1}        & \textbf{P}        & \textbf{R}         & \textbf{F1}        & \textbf{P}        & \textbf{R}         & \textbf{F1}         \\ 
\hline
%\rowcolor[rgb]{0.867,0.867,0.867} 
Sbert + MultiNFR\_A     & \textbf{0.24}         & \textbf{0.48}         & \textbf{0.32}         & 0.11                  & 0.10                  & 0.10                  & 0.09                  & 0.47                  & 0.15                  & 0.38                  & 0.23                  & 0.29                  & 0.04                  & 0.20                  & 0.07                   \\
%\rowcolor[rgb]{0.867,0.867,0.867} 
Sbert + MultiNFR\_B     & 0.20                  & 0.14                  & 0.17                  & \textit{0.00}           & \textit{0.00}           & \textit{0.00}           & \textbf{0.22}         & \textbf{\uline{0.71}} & \textbf{0.33}         & \textbf{\uline{0.67}} & \textbf{0.31}         & \textbf{\uline{0.42}} & \textbf{0.07}         & \textbf{\uline{0.50}} & \textbf{0.13}          \\
%\rowcolor[rgb]{0.867,0.867,0.867} 
Sbert + MultiNFR\_C     & 0.05                  & 0.14                  & 0.08                  & \textit{0.00}           & \textit{0.00}           & \textit{0.00}           & 0.09                  & 0.18                  & 0.12                  & 0.14                  & 0.23                  & 0.18                  & 0.09                  & 0.20                  & 0.12                   \\
%\rowcolor[rgb]{0.867,0.867,0.867} 
Sbert + MultiNFR\_D     & 0.15                  & 0.76                  & 0.25                  & \textbf{0.10}         & \textbf{0.24}         & \textbf{0.14}         & 0.08                  & 0.06                  & 0.07                  & 0.18                  & 0.15                  & 0.17                  & \textit{0.00}           & \textit{0.00}           & \textit{0.00}            \\
\hline
AllMini + MultiNFR\_A                                     & \textbf{\uline{0.27}} & \textbf{\uline{0.62}} & \textbf{\uline{0.38}} & \textbf{\uline{0.18}} & \textbf{\uline{0.86}} & \textbf{\uline{0.30}} & 0.24                  & 0.41                  & 0.30                  & 0.05                  & 0.08                  & 0.06                  & 0.07                  & 0.30                  & 0.11                   \\
AllMini + MultiNFR\_B                                     & 0.25                  & 0.33                  & 0.29                  & 0.13                  & 0.43                  & 0.21                  & \textbf{\uline{0.42}} & \textbf{0.47}         & \textbf{\uline{0.44}} & \textbf{0.20}         & \textbf{\uline{0.69}} & \textbf{0.32}         & 0.11                  & 0.60                  & 0.19                   \\
AllMini + MultiNFR\_C                                     & 0.12                  & 0.29                  & 0.17                  & 0.09                  & 0.62                  & 0.16                  & 0.07                  & 0.06                  & 0.06                  & \textbf{0.28}         & \textbf{0.38}         & \textbf{0.32}         & 0.50                  & 0.20                  & 0.29                   \\
AllMini + MultiNFR\_D                                     & 0.02                  & 0.05                  & 0.03                  & 0.12                  & 0.52                  & 0.19                  & 0.05                  & 0.05                  & 0.03                  & \textit{0.00}           & \textit{0.00}           & \textit{0.00}           & \textbf{\uline{1.00}} & \textbf{0.20}         & \textbf{\uline{0.33}}  \\
\hline
%\rowcolor[rgb]{0.867,0.867,0.867} 
Bert4RE + MultiNFR\_A   & \textit{0.00}           & \textit{0.00}           & \textit{0.00}           & \textit{0.00}                   & \textit{0.00}           & \textit{0.00}                    & \textbf{0.06}         & \textbf{0.94}         & \textbf{0.10}         & \textit{0.00}           & \textit{0.00}           & \textit{0.00}           & \textit{0.00}           & \textit{0.00}           & \textit{0.00}            \\
%\rowcolor[rgb]{0.867,0.867,0.867} 
Bert4RE + MultiNFR\_B   & \textit{0.00}           & \textit{0.00}           & \textit{0.00}           & 0.07                  & 0.10                  & 0.08                  & \textit{0.00}           & \textit{0.00}           & \textit{0.00}            & \textit{0.00}           & \textit{0.00}           & \textit{0.00}           & \textit{0.00}           & \textit{0.00}           & \textit{0.00}            \\
%\rowcolor[rgb]{0.867,0.867,0.867} 
Bert4RE + MultiNFR\_C   & \textbf{0.13}         & \textbf{0.05}         & \textbf{0.07}         & \textbf{0.07}         & \textbf{0.19}         & \textbf{0.10}         & \textit{0.00}           & \textit{0.00}           & \textit{0.00}          & \textit{0.00}           & \textit{0.00}           & \textit{0.00}           & \textit{0.00}           & \textit{0.00}           & \textit{0.00}            \\
%\rowcolor[rgb]{0.867,0.867,0.867} 
Bert4RE + MultiNFR\_D   & \textit{0.00}           & \textit{0.00}           & \textit{0.00}           & \textit{0.00}           & \textit{0.00}           & \textit{0.00}                    & 0.03                  & 0.06                  & 0.04                  & \textit{0.00}           & \textit{0.00}           & \textit{0.00}            & \textit{0.00}           & \textit{0.00}           & \textit{0.00}             \\
\hline
SObert + MultiNFR\_A                                      & \textit{0.00}           & \textit{0.00}           & \textit{0.00}           & \textit{0.00}           & \textit{0.00}           & \textit{0.00}           & \textit{0.00}           & \textit{0.00}           & \textit{0.00}            & \textit{0.00}           & \textit{0.00}           & \textit{0.00}          & \textit{0.00}           & \textit{0.00}           & \textit{0.00}           \\
SObert + MultiNFR\_B                                      & \textbf{0.08}         & \textbf{0.14}         & \textbf{0.10}         & \textit{0.00}           & \textit{0.00}           & \textit{0.00}            & \textit{0.00}           & \textit{0.00}           & \textit{0.00}          & \textbf{0.20}         & \textbf{0.08}         & \textbf{0.11}        & \textit{0.00}           & \textit{0.00}           & \textit{0.00}             \\
SObert + MultiNFR\_C                                      & \textit{0.00}           & \textit{0.00}           & \textit{0.00}         & \textit{0.00}           & \textit{0.00}           & \textit{0.00}          & 0.05                  & 0.41                  & 0.08                  & 0.02                  & 0.08                  & 0.03                  & \textbf{0.04}         & \textbf{0.10}         & \textbf{0.06}          \\
SObert + MultiNFR\_D                                      & \textit{0.00}           & \textit{0.00}           & \textit{0.00}           & \textbf{0.05}         & \textbf{0.60}         & \textbf{0.10}         & \textbf{0.08}         & \textbf{0.18}         & \textbf{0.11}         & \textit{0.00}           & \textit{0.00}           & \textit{0.00}        & \textit{0.00}           & \textit{0.00}           & \textit{0.00}          \\
\bottomrule
\end{tabular}
}
\end{table}
